# Supplementary material for: Convergence Properties of Dynamic Processes on Graphs
Source: arXiv:2406.05147 source file (2024-05-30)
Supplement: Supplementary file 1 [file z-appendix-1.tex]

\chapter{Appendix: Explanation on Appendices}\label{chap:appendix1}
