# Supplementary material for: Convergence Properties of Dynamic Processes on Graphs
Source: arXiv:2406.05147 source file (2024-05-30)
Supplement: Supplementary file 2 [file z-appendix-2.tex]

\chapter{Appendix: Explanation on Page Borders}\label{chap:appendix2}
